# Supplementary material for: Star formation in disk galaxies and its relation with spiral structure in numerical simulations
Source: arXiv:2204.08560 source file (2022-04-18)
Supplement: Supplementary file 1 [file AppendixA.tex]

% Appendix A

\chapter{Frequently Asked Questions} % Main appendix title

\label{AppendixA} % For referencing this appendix elsewhere, use \ref{AppendixA}

\section{How do I change the colors of links?}

The color of links can be changed to your liking using:

{\small\verb!\hypersetup{urlcolor=red}!}, or

{\small\verb!\hypersetup{citecolor=green}!}, or

{\small\verb!\hypersetup{allcolor=blue}!}.

\noindent If you want to completely hide the links, you can use:

{\small\verb!\hypersetup{allcolors=.}!}, or even better: 

{\small\verb!\hypersetup{hidelinks}!}.

\noindent If you want to have obvious links in the PDF but not the printed text, use:

{\small\verb!\hypersetup{colorlinks=false}!}.
