# Supplementary material for: Star formation in disk galaxies and its relation with spiral structure in numerical simulations
Source: arXiv:2204.08560 source file (2022-04-18)
Supplement: Supplementary file 2 [file AppendixTemplate.tex]

% Appendix Template

\chapter{Appendix Title Here} % Main appendix title

\label{AppendixX} % Change X to a consecutive letter; for referencing this appendix elsewhere, use \ref{AppendixX}

Write your Appendix content here.
